# Supplementary material for: Quantum Monte Carlo Calculations of neutron-$\alpha$ Scattering via an Integral Relation
Source: arXiv:2502.18718 source file (2025-02-26)
Supplement: Supplementary file 1 [file appendix.tex]

\appendix
